# Supplementary material for: On Diagnostics for Understanding Agent Training Behaviour in Cooperative MARL
Source: arXiv:2312.08468 source file (2023-12-13)
Supplement: Supplementary file 1 [file appendix.tex]

\newpage
\appendix

\section{ Experimental details}
\label{appendix:exp_details}

\subsection{Environments}

To ensure our experimentation setup is clear and easily reproducible, we make use of the same environment naming conventions used in \citep{papoudakis2021benchmarking}.
 In this section, we provide an overview of the naming conventions employed. Primarily we break down how the naming conventions of each environment correspond to the features of each scenario in the Level-Based Foraging (LBF) and Multi-Robot Warehouse (RWARE) environments.

Figure \ref{fig: all_envs_figures} illustrates a collection of ten scenarios, each corresponding to a specific task in the LBF and RWARE environments. The LBF scenarios are described in detail in Section \ref{LBF}, while the RWARE scenarios are explained in Section \ref{RWARE}.

\subsubsection{Level Based Foraging}  
\label{LBF}
\textbf{Naming Convention.} The scenarios in the LBF environment are named according to the following convention: 

\begin{center}
    Foraging<obs>-<x\_size>x<y\_size>-<n\_agents>p-<food>f<force\_c>-v1
\end{center}

Each field in the naming convention has specific options:
\begin{itemize}
\item <obs>: Denotes agent level of partial observability for all agents. If no value is given the agents can see as far as the grid is wide. 
\item <x\_size>: Size of the grid along the horizontal axis.
\item <y\_size>: Size of the grid along the vertical axis.
\item <n\_agents>: Number of agents in the environment.
\item <food>: Number of food items in the environment. This is the total number of food that can spawn per episode. 
\item <force\_c>: Optional field indicating a forced cooperative task. It can be empty or set to "-coop" mode. In this mode, the levels of all the food items are intentionally set equal to the sum of the levels of all the agents involved. This implies that the successful acquisition of a food item requires a high degree of cooperation between the agents since no agent will be able to collect a food item by itself. 

As an example, an environment named "Foraging-2s-8x8-2p-2f-coop" has a sight range of "2s" implying that agents can view a 5x5 grid centred on themselves, a grid with horizontal and vertical size 8, contains 2 agents, 2 food objects and is set to a cooperative mode.
\end{itemize}

\subsubsection{Used scenarios.} 
Our research experiments were carried out on a varied set of scenarios, and in all cases, agent positions and food positions as well as agent levels and food levels are randomly generated at each new environment episode.

\begin{itemize}
    \item Figure \ref{fig: all_envs_figures}(a) \textbf{Foraging-2s-8x8-2p-2f-coop}: 8x8 grid, partial observability with sight=2, 2 agents, 2 food items, cooperative mode.
      \item Figure \ref{fig: all_envs_figures}(b) \textbf{Foraging-8x8-2p-2f-coop}: 8x8 grid, full observability, 2 agents, 2 food items, cooperative mode.
      \item Figure \ref{fig: all_envs_figures}(c) \textbf{Foraging-2s-10x10-3p-3f}: 10x10 grid, partial observability, 3 agents, 3 food items.
      \item Figure \ref{fig: all_envs_figures}(d) \textbf{Foraging-10x10-3p-3f}: 10x10 grid, full observability, 3 agents, 3 food items.
      \item Figure \ref{fig: all_envs_figures}(e) \textbf{Foraging-15x15-3p-5f}: 15x15 grid, full observability, 3 agents, 5 food items.
      \item Figure \ref{fig: all_envs_figures}(f) \textbf{Foraging-15x15-4p-3f: 15x15 grid}, full observability, 4 agents, 3 food items.
      \item Figure \ref{fig: all_envs_figures}(g) \textbf{Foraging-15x15-4p-5f: 15x15 grid}, full observability, 4 agents, 5 food items.      
\end{itemize}

\subsubsection{Multi-Robot Warehouse} 
\label{RWARE}
\textbf{Naming Convention.} 
The scenarios in the RWARE environment are named according to the following convention: 
\begin{center}
    rware-<size>-<num\_agents>ag<diff>-v1
\end{center}
Each field in the naming convention has specific options:
\begin{itemize}
    \item <size>: Represents the size of the Warehouse (e.g., "tiny", "small", "medium",
    "large").
    \item <num\_agents>: Indicates the number of agents (1-20).
    \item <diff>: Optional field indicating the difficulty of the task (default: N requests for each of the N agents). 
\end{itemize}

\textbf{Used scenarios}
In this situation, the experiments in our study were carried out using three different scenarios of the RWARE environment.
In each of these scenarios, agents have a 3x3 observation grid centered on themselves, providing information on the location, rotation and surrounding configurations of other agents and shelves.
By default, the number of requested shelves is equal to the number of agents.

\begin{itemize}
    \item Figure \ref{fig: all_envs_figures}(h) \textbf{rware-tiny-2ag}: The tiny map is a grid world of 11x11 squares, partial observability, 2 agents.
    \item Figure \ref{fig: all_envs_figures}(i) \textbf{rware-tiny-4ag}: The tiny map is a grid world of 11x11 squares, partial observability, 4 agents.
    \item Figure \ref{fig: all_envs_figures}(j) \textbf{rware-small-4ag}: The small map is a grid world of 11x20 squares,
    partial observability, 4 agents.
\end{itemize}

% Figure for all envs images
\begin{figure}
  \centering
  \begin{subfigure}[t]{0.02\textwidth}
        \scriptsize
        \textbf{(a)}
 \end{subfigure}
  \begin{subfigure}[t]{0.2\linewidth}
    \includegraphics[width=\linewidth, valign=t]{figures/appendix/envs_plots/Foraging-2s-8x8-2p-2f-coop-v2.pdf}
  \end{subfigure}
  \begin{subfigure}[t]{0.02\textwidth}
        \scriptsize
        \textbf{(b)}
    \end{subfigure}
  \begin{subfigure}[t]{0.2\linewidth}
    \includegraphics[width=\linewidth, valign=t]{figures/appendix/envs_plots/Foraging-8x8-2p-2f-coop-v2.pdf}
  \end{subfigure}
  \begin{subfigure}[t]{0.02\textwidth}
        \scriptsize
        \textbf{(c)}
    \end{subfigure}
  \begin{subfigure}[t]{0.2\linewidth}
    \includegraphics[width=\linewidth, valign=t]{figures/appendix/envs_plots/Foraging-2s-10x10-3p-3f-v2.pdf}
  \end{subfigure}
  \begin{subfigure}[t]{0.02\textwidth}
        \scriptsize
        \textbf{(d)}
    \end{subfigure}
  \begin{subfigure}[t]{0.2\linewidth}
    \includegraphics[width=\linewidth, valign=t]{figures/appendix/envs_plots/Foraging-10x10-3p-3f-v2.pdf}
  \end{subfigure}\\
\begin{subfigure}[t]{0.02\textwidth}
        \scriptsize
        \textbf{(e)}
    \end{subfigure}
  \begin{subfigure}[t]{0.2\linewidth}
    \includegraphics[width=\linewidth, valign=t]{figures/appendix/envs_plots/Foraging-10x10-3p-3f-v2.pdf}
  \end{subfigure}
  \begin{subfigure}[t]{0.02\textwidth}
        \scriptsize
        \textbf{(f)}
    \end{subfigure}
  \begin{subfigure}[t]{0.2\linewidth}
    \includegraphics[width=\linewidth, valign=t]{figures/appendix/envs_plots/Foraging-15x15-4p-3f-v2.pdf}
  \end{subfigure}
    \begin{subfigure}[t]{0.02\textwidth}
        \scriptsize
        \textbf{(g)}
    \end{subfigure}
  \begin{subfigure}[t]{0.2\linewidth}
    \includegraphics[width=\linewidth, valign=t]{figures/appendix/envs_plots/Foraging-15x15-4p-5f-v2.pdf}
  \end{subfigure}
   \begin{subfigure}[t]{0.02\textwidth}
        \scriptsize
        \textbf{(h)}
    \end{subfigure}
  \begin{subfigure}[t]{0.2\linewidth}
    \includegraphics[width=\linewidth, valign=t]{figures/appendix/envs_plots/rware-tiny-2ag-v1.pdf}
  \end{subfigure}\\
\begin{subfigure}[t]{0.02\textwidth}
        \scriptsize
        \textbf{(i)}
    \end{subfigure}
  \begin{subfigure}[t]{0.2\linewidth}
    \includegraphics[width=\linewidth, valign=t]{figures/appendix/envs_plots/rware-tiny-4ag-v1.pdf}
  \end{subfigure}
  \begin{subfigure}[t]{0.02\textwidth}
        \scriptsize
        \textbf{(j)}
    \end{subfigure}
  \begin{subfigure}[t]{0.2\linewidth}
    \includegraphics[width=\linewidth,height=3.1cm, valign=t]{figures/appendix/envs_plots/rware-small-4ag-v1.pdf}
  \end{subfigure}
  \caption{\textit{Illustration of the seven LBF tasks and three RWARE tasks used for the main experiments.}}
  \label{fig: all_envs_figures}
\end{figure}

 \subsection{Algorithms Overview}
In our analysis, we restrict ourselves to a limited set of algorithms from MARL literature. Our algorithm selection is done to cover Q-learning and policy gradient (PG) based methods in both the independent learner  (IL) and centralised training decentralised execution (CTDE) paradigms. We also investigate the effect of parameter sharing and non-parameter sharing on the performance of the algorithms.

\subsubsection{Q-learning}
For Q-learning-based methods we have selected, VDN and QMIX which fall into the paradigm of \textbf{CTDE} and IQL which is an \textbf{IL} method.

\textbf{IQL:} For Independent Q-Learning (IQL) \citep{IQL}, each agent learns a policy based purely on their own egocentric experience in the training environment. This policy is parameterised by a Q-value network \citep{mnih2013playing}.

\textbf{VDN:} In Value-Decomposition Network (VDN) \citep{VDN}, IQL is extended through the use of value decomposition. Rather than learning purely from their own egocentric perspectives with each agent receiving the same reward, VDN formulates the joint Q value of the coalition as a linearly decomposed sum of the individual agent values. Each individual agent then updates its policy using the gradient flow based on a joint additive loss.

\textbf{QMIX}: \citep{QMIX} then extends VDN by broadening the range of reward functions that can be decomposed. To create a more complex attribution of the Q values, it makes use of a parameterised mixing network to perform the attribution. This mixing network takes the individual agent Q values as input and then policy updates are performed in an end-to-end manner where attribution is done using backpropagation. QMIX also allows the use of data augmentation by accommodating additional data at training time.

\subsubsection{Policy Gradients (PG)}

\textbf{IA2C:} Independent Advantage Actor-Critic (IA2C) is a variant of the A2C algorithm \citep{pmlr-v48-mniha16} applied to the multi-agent setting. IA2C trains agents using their own egocentric experiences in the training environment where each agent has their own critic and actor networks that approximate the optimal policy and state values.

\textbf{IPPO:} Independent Proximal Policy Optimisation (IPPO) is a variant of the PPO algorithm \citep{schulman2017proximal} applied to the multi-agent setting. PPO can be thought of as an improvement to A2C. It uses a surrogate objective that limits the change in the policy at each update step which allows the PPO to iterate over the same trajectory of data multiple times without policy divergence. Otherwise, its architecture is the same as A2C.

\textbf{MAPPO \& MAA2C:} Multi-Agent Proximal Policy Optimisation (MAPPO) and Multi-Agent Advantage Actor-Critic (MAA2C) \citep{yu2022surprising} extend IPPO and IA2C to make use of a joint state value function. Instead of multiple per-agent critics, there is a single critic that learns the value of the joint state representation rather than the egocentric individual agent observations. MAA2C is also sometimes referred to as Central-V \citep{foerster2018counterfactual} because of this but, to prevent confusion, we use MAA2C. MAPPO also makes use of the same CTDE type architecture with a centralised critic. 

\subsubsection{Parameter Sharing vs Non-Parameter Sharing:}
To improve sample efficiency it is common to use \textbf{Parameter Sharing} (PS) in cooperative MARL. When PS is in use, all of the agents on a team share the same set of parameters for their neural networks (NN). In practice, this is equivalent to using a single neural network to represent all members of the team. Typically a one-hot agent ID is added to the local observation of each agent so that the NN can determine which agent to behave as. In some cases, using PS limits performance as agents tend to learn a smaller subset of roles. Alternatively, we can use \textbf{concurrent/non-parameter shared} learning where each agent is represented by a different set of parameters. Under this paradigm, we train each agent's parameters concurrently and maintain separate parameters for each individual agent.

\subsubsection{Experimental Hyperparameters}
In our analysis, we sought to conduct comprehensive experiments in various environments using different algorithms. To ensure reliable and consistent results, it is important to carefully select and optimise the hyperparameters for each algorithm in each environment.

To this end, we used the optimised hyperparameters from \cite{papoudakis2021benchmarking}, where the parameters of each algorithm were chosen based on a hyperparameter sweep for a single scenario of each environment and then reused across all other scenarios for the same settings. The choice of the set of hyperparameters is done by selecting the one with the highest evaluation score averaged over three seeds.

Tables \ref{tab: q_learning_hyperparams} and \ref{tab: pg_hyperparams} provide a summary of the shared hyperparameters used in the Q-learning and policy gradient algorithms, respectively. On the other hand, Tables \ref{tab: iql_hyperparams}, \ref{tab: vdn_hyperparams}, and \ref{tab: qmix_hyperparams} specify the algorithm-specific hyperparameters for each Q-learning algorithm, namely IQL, VDN, and QMIX, respectively. Similarly, Tables \ref{tab: mappo_hyperparams} and \ref{tab: maa2c_hyperparams} present the specific hyperparameter settings for the policy-gradient algorithms, namely MAPPO and MAA2C, respectively. 

These aforementioned tables offer an overview of the hyperparameters utilised in each environment, encompassing the applicable algorithms in both parameter-sharing and non-parameter-sharing scenarios.

% Q-learning tables:
\begin{table}
  \centering
  \caption{Shared hyperparameters for Q-learning algorithms with and  without parameter sharing}
  \label{tab: q_learning_hyperparams}
  
  \setlength{\heavyrulewidth}{1.5pt}
  \setlength{\abovetopsep}{4pt}
  \begin{tabular}{ccccp{2cm}}
    \toprule
    & \multicolumn{1}{c}{\textbf{Parameter Sharing}} & \multicolumn{1}{c}{\textbf{Non-Parameter Sharing}} \\
    \midrule
    Optimizer &Adam & Adam \\ 
    Maximum gradient norm & 10 & 10\\
    Reward standardisation & True & True \\
    Network type & GRU  & GRU \\
    Discount factor & 0.99 & 0.99 \\
    $\epsilon$ schedule steps & 2e6 &  5e4\\
    $\epsilon$ schedule minimum & 0.05 & 0.05\\
    Batch size & 32 & 32 \\
    Replay buffer size & 5000 & 5000 \\
    Parallel workers & 1 & 1\\
    \bottomrule
  \end{tabular}
\end{table}

\begin{table}
  \centering
  \caption{Shared hyperparameters for IQL with and  without parameter sharing}
  \label{tab: iql_hyperparams}
  
  \setlength{\heavyrulewidth}{1.5pt}
  \setlength{\abovetopsep}{4pt}
  \begin{tabular}{ccccp{2cm}}
    \toprule
    & \multicolumn{1}{c}{\textbf{Parameter Sharing}} & \multicolumn{1}{c}{\textbf{Non-Parameter Sharing}} \\
    \midrule
    Hidden dimension & 128 & 64\\
    Learning rate & 0.0003 & 0.0003 \\
    Reward standardisation & True & True \\
    Network type & GRU & GRU \\
    Evaluation epsilon & 0.05 & 0.05 \\
    Target update & 200(hard) & 200(hard) \\
    \bottomrule
  \end{tabular}
\end{table}

\begin{table}
  \centering
  \caption{Hyperparameters for VDN with and  without parameter sharing}
  \label{tab: vdn_hyperparams}
  
  \setlength{\heavyrulewidth}{1.5pt}
  \setlength{\abovetopsep}{4pt}
  \begin{tabular}{ccccp{2cm}}
    \toprule
    & \multicolumn{1}{c}{\textbf{Parameter Sharing}} & \multicolumn{1}{c}{\textbf{Non-Parameter Sharing}} \\
    \midrule
    Hidden dimension & 128 & 64 &\\
    Learning rate & 0.0003 & 0.0001 \\
    Reward standardisation & True & True \\
    Network type & GRU & GRU \\
    Evaluation epsilon & 0.0 & 0.05 \\
    Target update & 0.01(\textbf{soft}) & 200(\textbf{hard}) \\
    \bottomrule
  \end{tabular}
\end{table}

\begin{table}
  \centering
  \caption{Hyperparameters for QMIX with and  without parameter sharing}
  \label{tab: qmix_hyperparams}
  
  \setlength{\heavyrulewidth}{1.5pt}
  \setlength{\abovetopsep}{4pt}
  \begin{tabular}{ccccp{2cm}}
    \toprule
    & \multicolumn{2}{c}{\textbf{Parameter Sharing}} & \multicolumn{2}{c}{\textbf{Non-Parameter Sharing}} \\
    \cmidrule(lr){2-3} \cmidrule(l){4-5}
    & \textbf{LBF} & \textbf{RWARE} & \textbf{LBF} & \textbf{RWARE} \\
    \midrule
    Hidden dimension & 64 & 64 & 64 & 64 \\
    Network type & GRU & FC & GRU & FC\\
    Mixing network size & 32 & 32& 32 & 32\\
    Mixing network type & FC &FC & FC & FC\\
    Mixing network activation & ReLU & ReLU & ReLU & ReLU\\
    Hypernetwork size & 64 & 64 & 64 & 64\\
    Hypernetwork activation & ReLU & ReLU & ReLU & ReLU\\
    Hypernetworks layers& 2&2&2&2\\
    Learning rate & 0.0003 & 0.0005 & 0.0001 & 0.0003 \\
    Reward standardisation & True & True  & True & True\\
    Evaluation epsilon & 0.05 & 0.05 & 0.05 & 0.05 \\
    Target update & 0.01(\textbf{soft}) & 0.01(\textbf{soft}) & 0.01 (\textbf{soft}) & 0.01 (\textbf{soft}) \\
    \bottomrule
  \end{tabular}
\end{table}

% Policy gradient tables:

\begin{table}
  \centering
  \caption{Shared hyperparameters for Policy-based algorithms with and  without parameter sharing}
  \label{tab: pg_hyperparams}
  
  \setlength{\heavyrulewidth}{1.5pt}
  \setlength{\abovetopsep}{4pt}
  \begin{tabular}{ccccp{2cm}}
    \toprule
    & \multicolumn{2}{c}{\textbf{Parameter Sharing}} & \multicolumn{2}{c}{\textbf{Non-Parameter Sharing}} \\
    \cmidrule(lr){2-3} \cmidrule(l){4-5}
    & \textbf{LBF} & \textbf{RWARE} & \textbf{LBF} & \textbf{RWARE} \\
    \midrule
    Optimizer &Adam & Adam & Adam & Adam \\ 
    Maximum gradient norm & 10 & 10 & 10 & 10\\
    Discount factor & 0.99 & 0.99 & 0.99 & 0.99\\
    Entropy coefficient & 0.001 & 0.001 & 0.001 & 0.001\\
    Batch size & 10 & 10 & 10 & 10\\
    Replay buffer size & 10 & 10 & 10 & 10\\
    Parallel workers & 10 & 10 & 10 & 10\\
    \bottomrule
  \end{tabular}
\end{table}

\begin{table}
  \centering
  \caption{Hyperparameters for MAPPO with and  without parameter sharing}
  \label{tab: mappo_hyperparams}
  
  \setlength{\heavyrulewidth}{1.5pt}
  \setlength{\abovetopsep}{4pt}
  \begin{tabular}{ccccp{2cm}}
    \toprule
    & \multicolumn{2}{c}{\textbf{Parameter Sharing}} & \multicolumn{2}{c}{\textbf{Non-Parameter Sharing}} \\
    \cmidrule(lr){2-3} \cmidrule(l){4-5}
    & \textbf{LBF} & \textbf{RWARE} & \textbf{LBF} & \textbf{RWARE} \\
    \midrule
    Hidden dimension & 128 & 128 & 128 & 128 \\
    Learning rate & 0.0003 & 0.0005 & 0.0001 & 0.0005 \\
    Reward standardisation & False & False  & False & False\\
    Network type & FC & FC & FC & FC\\
    Evaluation epsilon & 0.05 & 0.05 & 0.05 & 0.05 \\
    Epsilon clip & 0.2 & 0.2 & 0.2 & 0.2 \\
    Epochs & 4 & 4 & 4 & 4 \\
    Target update & 0.01(soft) & 0.01(soft) & 200 (hard) & 0.01 (soft) \\
    n-step & 5 & 10 & 10 & 10\\
    \bottomrule
  \end{tabular}
\end{table}

\begin{table}
  \centering
  \caption{Hyperparameters for MAA2C with and  without parameter sharing}
  \label{tab: maa2c_hyperparams}
  
  \setlength{\heavyrulewidth}{1.5pt}
  \setlength{\abovetopsep}{4pt}
  \begin{tabular}{ccccp{2cm}}
    \toprule
    & \multicolumn{2}{c}{\textbf{Parameter Sharing}} & \multicolumn{2}{c}{\textbf{Non-Parameter Sharing}} \\
    \cmidrule(lr){2-3} \cmidrule(l){4-5}
    & \textbf{LBF} & \textbf{RWARE} & \textbf{LBF} & \textbf{RWARE} \\
    \midrule
    Hidden dimension & 128 & 64 & 128 & 64 \\
    Learning rate & 0.0005 & 0.0005 & 0.0005 & 0.0005 \\
    Reward standardisation & True & True  & True & True\\
    Network type & GRU & FC & GRU & FC\\
    Evaluation epsilon & 0.01 & 0.01 & 0.01 & 0.01 \\
    Target update & 0.01(soft) & 0.01(soft) & 0.01 (soft) & 0.01 (soft) \\
    n-step & 10 & 5 & 5 & 5\\
    \bottomrule
  \end{tabular}
\end{table}

\section{Parameter sharing Experiments}
\label{sec: param_share_exp}

In this section, we present additional plots that complement the figures presented in the main paper. In Figure \ref{fig: shared_all_tasks}, we can observe the performance of the aforementioned algorithms in the seven LBF tasks and the 3 RWARE tasks where we recorded the results of Mean episode returns with the mean and 95\% confidence intervals over 10 distinct seeds in the 201 evaluations.

% All task plots for the shared case
\begin{figure}[ht!]
  \centering
    \begin{subfigure} {1\linewidth}
    \includegraphics[width=\linewidth]{figures/appendix/shared_params/shared_all_tasks.pdf} 
    \end{subfigure}
    
    \begin{subfigure} {0.3\linewidth}
    \includegraphics[width=\linewidth]{figures/appendix/shared_params/rest_shared_all_tasks.pdf}
    \end{subfigure}
  \caption{Mean episode returns for all algorithms with parameter sharing in seven LBF scenarios and three RWARE scenarios, with the mean and 95\% confidence intervals over 10 distinct seeds.}
  \label{fig: shared_all_tasks}
  
\end{figure}

\subsubsection{Additional Metric Results}
In this section, we present the results of applying the Policy Entropy, Agent Update Divergence, and Task Switching tools to five different algorithms in the "Foraging-2s-10x10-3p-3f-v2" scenario, where agents have limited observations of the environment. The results are shown in Figures \ref{fig:app_entropy} to \ref{fig:app_ts}, where each plot displays the values of the metrics for each agent and their average across all agents.

%KL plots
\begin{figure}[ht!]
    \centering
    \begin{subfigure}[b]{0.3\textwidth}
        \includegraphics[width=\textwidth]{figures/appendix/shared_params/stability/Foraging-2s-10x10-3p-3f-v2/0_maa2c_kl_divergence.pdf}
        \caption{MAA2C}
        \label{fig:maa2c_kl_div}
    \end{subfigure}
    \begin{subfigure}[b]{0.3\textwidth}
        \includegraphics[width=\textwidth]{figures/appendix/shared_params/stability/Foraging-2s-10x10-3p-3f-v2/0_mappo_kl_divergence.pdf}
        \caption{MAPPO}
        \label{fig:mappo_kl_div}
    \end{subfigure}
    \begin{subfigure}[b]{0.3\textwidth}
        \includegraphics[width=\textwidth]{figures/appendix/shared_params/stability/Foraging-2s-10x10-3p-3f-v2/0_iql_kl_divergence.pdf}
        \caption{IQL}
        \label{fig:iql_kl_div}
    \end{subfigure}
    \begin{subfigure}[b]{0.3\textwidth}
        \includegraphics[width=\textwidth]{figures/appendix/shared_params/stability/Foraging-2s-10x10-3p-3f-v2/0_qmix_kl_divergence.pdf}
        \caption{QMIX}
        \label{fig:qmix_kl_div}
    \end{subfigure}
    \begin{subfigure}[b]{0.3\textwidth}
        \includegraphics[width=\textwidth]{figures/appendix/shared_params/stability/Foraging-2s-10x10-3p-3f-v2/0_vdn_kl_divergence.pdf}
        \caption{VDN}
        \label{fig:vdn_kl_div}
    \end{subfigure}
    \caption{\textit{Agent Update Divergence results on \texttt{Foraging-10x10-3p-3f-v2} (one seed)}.}
    \label{fig:app_entropy}
\end{figure}

%Entropy plots
\begin{figure}[ht!]
    \centering
     \begin{subfigure}[b]{0.3\textwidth}
        \includegraphics[width=\textwidth]{figures/appendix/shared_params/stability/Foraging-2s-10x10-3p-3f-v2/0_maa2c_joint_action_entropy.pdf}
        \caption{MAA2C}
        \label{fig:maa2c_entropy}
    \end{subfigure}
     \begin{subfigure}[b]{0.3\textwidth}
        \includegraphics[width=\textwidth]{figures/appendix/shared_params/stability/Foraging-2s-10x10-3p-3f-v2/0_mappo_joint_action_entropy.pdf}
        \caption{MAPPO}
        \label{fig:mappo_entropy}
    \end{subfigure}
    \begin{subfigure}[b]{0.3\textwidth}
        \includegraphics[width=\textwidth]{figures/appendix/shared_params/stability/Foraging-2s-10x10-3p-3f-v2/0_iql_joint_action_entropy.pdf}
        \caption{IQL}
        \label{fig:iql_entropy}
    \end{subfigure}
    \begin{subfigure}[b]{0.3\textwidth}
        \includegraphics[width=\textwidth]{figures/appendix/shared_params/stability/Foraging-2s-10x10-3p-3f-v2/0_qmix_joint_action_entropy.pdf}
        \caption{QMIX}
        \label{fig:qmix_entropy}
    \end{subfigure}
    \begin{subfigure}[b]{0.3\textwidth}
        \includegraphics[width=\textwidth]{figures/appendix/shared_params/stability/Foraging-2s-10x10-3p-3f-v2/0_vdn_joint_action_entropy.pdf}
        \caption{VDN}
        \label{fig:vdn_entropy}
    \end{subfigure}
    \caption{\textit{Policy Entropy results on \texttt{Foraging-2s-10x10-3p-3f} (one seed)}.}
    \label{fig:app_kl}
\end{figure}

%Task switching
\begin{figure}[ht!]
    \centering
    \begin{subfigure}{0.85\textwidth}
        \includegraphics[width=\textwidth]{figures/appendix/shared_params/ts/Foraging-2s-10x10-3p-3f-v2/0_maa2c_Foraging-2s-10x10-3p-3f-v2_task_switching.pdf}
    \end{subfigure}
    \begin{subfigure}{0.85\textwidth}
        \includegraphics[width=\textwidth]{figures/appendix/shared_params/ts/Foraging-2s-10x10-3p-3f-v2/0_mappo_Foraging-2s-10x10-3p-3f-v2_task_switching.pdf}
    \end{subfigure}
    \begin{subfigure}{0.85\textwidth}
        \includegraphics[width=\textwidth]{figures/appendix/shared_params/ts/Foraging-2s-10x10-3p-3f-v2/0_iql_Foraging-2s-10x10-3p-3f-v2_task_switching.pdf}
    \end{subfigure}
    \begin{subfigure}{0.85\textwidth}
        \includegraphics[width=\textwidth]{figures/appendix/shared_params/ts/Foraging-2s-10x10-3p-3f-v2/0_qmix_Foraging-2s-10x10-3p-3f-v2_task_switching.pdf}
    \end{subfigure}
    \begin{subfigure}{0.85\textwidth}
        \includegraphics[width=\textwidth]{figures/appendix/shared_params/ts/Foraging-2s-10x10-3p-3f-v2/0_vdn_Foraging-2s-10x10-3p-3f-v2_task_switching.pdf}
    \end{subfigure}
    \caption{\textit{Task Switching on \texttt{Foraging-10x10-3p-3f-v2} (one seed)}. Each row corresponds to a different algorithm: MAA2C, MAPPO, IQL, QMIX, and VDN. }
    \label{fig:app_ts}
\end{figure}

\subsection{Non Parameter sharing Experiments}
\label{appendix:ns_shared}
In this section, we present the results of applying the non-parameter sharing (NPS) approach to the LBF scenarios, where agents have different observation spaces and action spaces. The NPS approach allows each agent to have its own neural network and learn its own policy independently, without sharing any parameters or gradients with other agents. We compare the performance of five different algorithms that use the NPS approach: IQL, QMIX, VDN, MAA2C, and MAPPO. We measure their performance using the aggregate score metric, which is the sum of the rewards obtained by all agents in an episode.

The results are shown in Figure \ref{fig:app_nonn_shared_benchmarking_paper_redo}, where each plot displays the aggregate score curves for each algorithm and their average across 10 seeds. We can observe that MAA2C and MAPPO achieve significantly higher aggregate scores than IQL, QMIX, and VDN in both LBF and RWARE scenarios. This suggests that MAA2C and MAPPO are able to learn more effective in these scenarios than IQL, QMIX, and VDN.

% Samples efficiency curves
\begin{figure}[ht!]
    \centering
    \includegraphics[width=0.7\textwidth]{figures/appendix/non_shared/legend_non_shared.pdf}
    \includegraphics[width=0.45\textwidth]{figures/appendix/non_shared/lbforaging_probability_of_improvement.pdf}
    \includegraphics[width=0.45\textwidth]{figures/appendix/non_shared/lbforaging_sample_efficiency_curves.pdf}
    \includegraphics[width=0.45\textwidth]{figures/appendix/non_shared/rware_probability_of_improvement.pdf}
    \includegraphics[width=0.45\textwidth]{figures/appendix/non_shared/rware_sample_efficiency_curves.pdf}
    \caption{\textit{Algorithm performance on LBF and RWARE including probability of improvement(left), and sample efficiency curves(right)}. \textbf{Top row:} Performance of algorithms on 7 LBF tasks. \textbf{Bottom row:} Performance of all algorithms on 3 RWARE tasks.}
    \label{fig:app_nonn_shared_benchmarking_paper_redo}
\end{figure}

\subsubsection{Additional Metric Results}
In this section, we present the results of applying the Policy Entropy, Agent Update Divergence, and Task Switching tools to the five algorithms that use the NPS approach in the LBF scenarios. The results are shown in Figures \ref{fig:ns_kl} to \ref{fig:ns_ts}, where each plot displays the values of the metrics for each agent and their average across all agents.

%KL plots
\begin{figure}[ht!]
    \centering
    \begin{subfigure}[b]{0.3\textwidth}
        \includegraphics[width=\textwidth]{figures/appendix/non_shared/stability/0_maa2c_ns_kl_divergence.pdf}
        \caption{MAA2C}
        \label{fig:maa2c_ns_kl_div}
    \end{subfigure}
    \begin{subfigure}[b]{0.3\textwidth}
        \includegraphics[width=\textwidth]{figures/appendix/non_shared/stability/0_mappo_ns_kl_divergence.pdf}
        \caption{MAPPO}
    \end{subfigure}
    \begin{subfigure}[b]{0.3\textwidth}
        \includegraphics[width=\textwidth]{figures/appendix/non_shared/stability/0_iql_ns_kl_divergence.pdf}
        \caption{IQL}
        \label{fig:iql_ns_kl_div}
    \end{subfigure}
    \begin{subfigure}[b]{0.3\textwidth}
        \includegraphics[width=\textwidth]{figures/appendix/non_shared/stability/0_qmix_ns_kl_divergence.pdf}
        \caption{QMIX}
        \label{fig:qmix_ns_kl_div}
    \end{subfigure}
    \begin{subfigure}[b]{0.3\textwidth}
        \includegraphics[width=\textwidth]{figures/appendix/non_shared/stability/0_vdn_ns_kl_divergence.pdf}
        \caption{VDN}
    \end{subfigure}
    \caption{\textit{Agent Update Divergence results on \texttt{Foraging-15x15-3p-5f} without parameter sharing (one seed)}.}
    \label{fig:ns_kl}
\end{figure}

% Entropy plots
\begin{figure}[ht!]
    \centering
    \begin{subfigure}[b]{0.3\textwidth}
        \includegraphics[width=\textwidth]{figures/appendix/non_shared/stability/0_maa2c_ns_joint_action_entropy.pdf}
        \caption{MAA2C}
        \label{fig:maa2c_entropy}
    \end{subfigure}
     \begin{subfigure}[b]{0.3\textwidth}
        \includegraphics[width=\textwidth]{figures/appendix/non_shared/stability/0_mappo_ns_joint_action_entropy.pdf}
        \caption{MAPPO}
        \label{fig:mappo_entropy}
    \end{subfigure}
    \begin{subfigure}[b]{0.3\textwidth}
        \includegraphics[width=\textwidth]{figures/appendix/non_shared/stability/0_iql_ns_joint_action_entropy.pdf}
        \caption{IQL}
        \label{fig:iql_entropy}
    \end{subfigure}
    \begin{subfigure}[b]{0.3\textwidth}
        \includegraphics[width=\textwidth]{figures/appendix/non_shared/stability/0_qmix_ns_joint_action_entropy.pdf}
        \caption{QMIX}
        \label{fig:qmix_entropy}
    \end{subfigure}
    \begin{subfigure}[b]{0.3\textwidth}
        \includegraphics[width=\textwidth]{figures/appendix/non_shared/stability/0_vdn_ns_joint_action_entropy.pdf}
        \caption{VDN}
        \label{fig:qmix_entropy}
    \end{subfigure}
    \caption{\textit{Policy Entropy results on \texttt{Foraging-15x15-3p-5f} without parameter sharing (one seed)}.}
    \label{fig:ns_entropy}
\end{figure}

% Task Switching plots IQL vs. Value-Decomposition plots
\begin{figure}[ht!]
    \centering
    \begin{subfigure}{0.85\textwidth}
        \includegraphics[width=\textwidth]{figures/appendix/non_shared/ts/0_maa2c_Foraging-15x15-3p-5f-v2_task_switching.pdf}
    \end{subfigure}
    \hfill
    \begin{subfigure}{0.85\textwidth}
        \includegraphics[width=\textwidth]{figures/appendix/non_shared/ts/0_mappo_Foraging-15x15-3p-5f-v2_task_switching.pdf}
    \end{subfigure}
    \begin{subfigure}{0.85\textwidth}
        \includegraphics[width=\textwidth]{figures/appendix/non_shared/ts/0_iql_Foraging-15x15-3p-5f-v2_task_switching.pdf}
    \end{subfigure}
    \hfill
    \begin{subfigure}{0.85\textwidth}
        \includegraphics[width=\textwidth]{figures/appendix/non_shared/ts/0_qmix_Foraging-15x15-3p-5f-v2_task_switching.pdf}
    \end{subfigure}
    \begin{subfigure}{0.85\textwidth}
        \includegraphics[width=\textwidth]{figures/appendix/non_shared/ts/0_vdn_Foraging-15x15-3p-5f-v2_task_switching.pdf}
    \end{subfigure}
    \caption{\textit{Task Switching on \texttt{Foraging-15x15-3p-5f} without parameter sharing (one seed)}. Each row corresponds to a
different algorithm: MAA2C, MAPPO, IQL, QMIX, and VDN.}
    \label{fig:ns_ts}
\end{figure}
